# Supplementary material for: S2O: Static to Openable Enhancement for Articulated 3D Objects
Source: arXiv:2409.18896 source file (2025-03-15)
Supplement: Supplementary file 1 [file supplemental.tex]

\documentclass[10pt,twocolumn,letterpaper]{article}
\usepackage[review]{cvpr} \input{macros.tex}

\begin{document}
\title{\papertitle{} Supplemental Materials}
\maketitle

\appendix

\title{\papertitle{} Supplemental Materials}
\maketitle

\appendix

{
\small
\bibliographystyle{ieeenat_fullname}
\bibliography{main}
}

{
\small
\bibliographystyle{ieeenat_fullname}
\bibliography{main}
}

\end{document}
